# Supplementary material for: Yang-Baxter integrable open quantum systems
Source: arXiv:2312.00064 source file (2023-11-29)
Supplement: Supplementary file 1 [file appendix1.tex]

%!TEX root = ../thesis.tex
% ******************************* Thesis Appendix A ****************************
\chapter{$R$-matrix for model B2}
\red{PLS do not read this appendix}

\label{RforB2}
\green{Be careful beause the following is for $\phi=0$ and $ch(u)\to cos(2v)$ and $i sh(u)\to -sin(2v)$}

The $R$-matrix for the model characterized by the Hamiltonian \eqref{hurapdep3} can be found by the Shastry $R$-matrix, \green{cite Hubbard Korepin book}.\\
In order to map the two models, one needs to allow some transformations that preserve integrability. In particular by starting from the $R$ 
\begin{itemize}
\item[1.] a local basis transformation $L$
\item[2.] two Drinfeld twists $A, B$
\item [3.] a local basis transformation $U$
\item [4.] a renormalization $\mathcal{N}$
\end{itemize}
\green{probably things can be simplified, or if you want we can also remove the details on the transformations and kust leave the answer}

Explicitly
\begin{align}
R_{B2}=\mathcal{N}(\mu,\nu)\big( U(\mu)\otimes U(\nu)\big) A(\mu,\nu) (L\otimes L) R_{Shastry} (L\otimes L)^{-1} B(\mu,v) \big( U(\mu)\otimes U(\nu)\big)^{-1}
\end{align}
where
\begin{align}
&L=\left(
\begin{array}{cccc}
 1 & 0 & 0 & 0 \\
 0 & 0 & 0 & 1 \\
 0 & 0 & 1 & 0 \\
 0 & 1 & 0 & 0 \\
\end{array}
\right),
&&U(\mu)=\left(
\begin{array}{cccc}
 0 & e^{\frac{1}{2} \sinh ^{-1}(\gamma  \sin (2 \mu))} & 0 & 0 \\
 e^{\frac{1}{2} \sinh ^{-1}(\gamma  \sin (2 \mu))} & 0 & 0 & 0 \\
 0 & 0 & 1 & 0 \\
 0 & 0 & 0 & 1 \\
\end{array}
\right)
\end{align}
$A(u,v)$ and $B(u,v)$ are diagonal matrices with elements
\begin{align}
&A=\left\{f_1,1,-1,1,1,1,1,1,1,1,1,f_2,-1,1,f_3,1\right\}\\
&B=\left\{f_1^{-1},1,1,-1,1,1,1,1,-1,1,1,f_2^{-1},1,1,f_3^{-1},1\right\}
\end{align}
\begin{align}
&f_1=e^{\frac{E\left(2 \mu\left|-\gamma ^2\right.\right)-\left(\gamma ^2+1\right) F\left(2 \mu\left|-\gamma ^2\right.\right)}{\gamma }},\\
&f_2=e^{\sinh ^{-1}(\gamma  \sin (2 \mu))} \left(\sqrt{\gamma ^2+2-\gamma ^2 \cos (4 \mu)}-\sqrt{2} \gamma  \sin (2 \mu)\right),\\
&f_3=e^{\sinh ^{-1}(\gamma  \sin (2 \mu))} \left(\sqrt{2} \gamma  \sin (2 \mu)-\sqrt{\gamma ^2+\gamma ^2 (-\cos (4 \mu))+2}\right)\\
\mathcal{N}(\mu,\nu)=&-\frac{\sqrt{2} \gamma  \mu  \cos ^2(2 \nu ) \left(-2 \gamma -\text{E}_{\nu }+\left(\gamma ^2+1\right) F_{\nu }\right)}{\sqrt{2} \gamma ^2 \nu  (\cos (4 \nu )+1)+\text{E}_{\nu } \sqrt{\gamma ^2 (-\cos (4 \nu ))+\gamma ^2+2}-\left(\gamma ^2+1\right) F_{\nu } \sqrt{\gamma ^2 (-\cos (4 \nu ))+\gamma ^2+2}}\\
&-\frac{\left(1-\frac{\sqrt{2} \gamma  \nu  \cos ^2(2 \nu )}{\sqrt{\gamma ^2 (-\cos (4 \nu ))+\gamma ^2+2}}\right) \left(\left(\gamma ^2+1\right) F_\mu-\text{E}_{\mu }\right)}{2 \left(\frac{\sqrt{2} \gamma ^2 \nu  \cos ^2(2 \nu )}{\sqrt{\gamma ^2 (-\cos (4 \nu ))+\gamma ^2+2}}+\frac{1}{2} \left(\text{E}_{\nu }-\left(\gamma ^2+1\right) F_{\nu }\right)\right)},
\end{align}
where we used the shortcut $E_\mu \to E(2 \mu ,-\gamma ^2)$.\\
We emphatize that $A\neq B^{-1}$ and the reason is that the $R$ matrix of the Hubbard model is graded. The differences in signs can be considered a map to un-graded $R$.\green{is it correct?}

Furthermore, the coupling constants should be mapped in this way\footnote{To be precise one needs to chose the branch such that \begin{align}
&\Big( \frac{\gamma }{\sqrt{\gamma ^2+\gamma ^2 (-\cos (4 v))+2}}\Big)_{Shastry}\to -\Big(\frac{1}{\sqrt{u-\cos (4 v)}}\Big)_{B2}
\end{align}}
\begin{align}
&\Big(\frac{\gamma ^2+2 }{\gamma^2}\Big)_{Shastry}\to\Big( u\Big)_{B2}.
\end{align}
Explicitly the $R$-matrix is
\begin{align}
&\mathcal{N}\rho_4\left(
\begin{array}{cccccccccccccccc}
 \rho _1 & 0 & 0 & 0 & 0 & 0 & 0 & 0 & 0 & 0 & 0 & 0 & 0 & 0 & 0 & 0 \\
 0 & \rho _3 & 0 & 0 & -\rho _8 & 0 & 0 & 0 & 0 & 0 & 0 & g_2 \rho _6 & 0 & 0 & g_2 \rho _6 & 0 \\
 0 & 0 & 1 & 0 & 0 & 0 & 0 & 0 & g_4 \rho _9 & 0 & 0 & 0 & 0 & 0 & 0 & 0 \\
 0 & 0 & 0 & 1 & 0 & 0 & 0 & 0 & 0 & 0 & 0 & 0 & g_4 \rho _9 & 0 & 0 & 0 \\
 0 & -\rho _8 & 0 & 0 & \rho _3 & 0 & 0 & 0 & 0 & 0 & 0 & g_2 \rho _6 & 0 & 0 & g_2 \rho _6 & 0 \\
 0 & 0 & 0 & 0 & 0 & \rho _1 & 0 & 0 & 0 & 0 & 0 & 0 & 0 & 0 & 0 & 0 \\
 0 & 0 & 0 & 0 & 0 & 0 & -1 & 0 & 0 & -g_4 \rho _9 & 0 & 0 & 0 & 0 & 0 & 0 \\
 0 & 0 & 0 & 0 & 0 & 0 & 0 & -1 & 0 & 0 & 0 & 0 & 0 & -g_4 \rho _9 & 0 & 0 \\
 0 & 0 & g_3 \rho _{10} & 0 & 0 & 0 & 0 & 0 & 1 & 0 & 0 & 0 & 0 & 0 & 0 & 0 \\
 0 & 0 & 0 & 0 & 0 & 0 & -g_3 \rho _{10} & 0 & 0 & -1 & 0 & 0 & 0 & 0 & 0 & 0 \\
 0 & 0 & 0 & 0 & 0 & 0 & 0 & 0 & 0 & 0 & \rho _4 & 0 & 0 & 0 & 0 & 0 \\
 0 & g_1 \rho _6 & 0 & 0 & g_1 \rho _6 & 0 & 0 & 0 & 0 & 0 & 0 & -\rho _5 & 0 & 0 & \rho _7 & 0 \\
 0 & 0 & 0 & g_3 \rho _{10} & 0 & 0 & 0 & 0 & 0 & 0 & 0 & 0 & 1 & 0 & 0 & 0 \\
 0 & 0 & 0 & 0 & 0 & 0 & 0 & -g_3 \rho _{10} & 0 & 0 & 0 & 0 & 0 & -1 & 0 & 0 \\
 0 & g_1 \rho _6 & 0 & 0 & g_1 \rho _6 & 0 & 0 & 0 & 0 & 0 & 0 & \rho _7 & 0 & 0 & -\rho _5 & 0 \\
 0 & 0 & 0 & 0 & 0 & 0 & 0 & 0 & 0 & 0 & 0 & 0 & 0 & 0 & 0 & \rho _4 \\
\end{array}
\right),
\end{align}
where the $\rho$s are defined in Shastry book. For completeness we will report here

\green{I wrote everything in terms of $\gamma$ because it looked a little nicer, if we write in terms of $u$ many square root appear}

\begin{align}
&\rho_1=e^{l-h} \sin (\mu ) \sin (\nu )+e^{h-l} \cos (\mu ) \cos (\nu ),
&\rho_3=\frac{e^{h-l} \cos (\mu ) \cos (\nu )-e^{l-h} \sin (\mu ) \sin (\nu )}{\cos ^2(\mu )-\sin ^2(\nu )}\\
&\rho_4=e^{h-l} \sin (\mu ) \sin (\nu )+e^{l-h} \cos (\mu ) \cos (\nu )
&\rho_5=\frac{e^{l-h} \cos (\mu ) \cos (\nu )-e^{h-l} \sin (\mu ) \sin (\nu )}{\cos ^2(\mu )-\sin ^2(\nu )}\\
&\rho_6=\frac{\sinh (2 (h-l))}{2 u \left(\cos ^2(\mu )-\sin ^2(\nu )\right)},
&\rho_7=\rho_4-\rho_5, \,\,\rho_8= \rho_1-\rho_3\\
&\rho_9=e^{l-h} \sin (\mu ) \cos (\nu )-e^{h-l} \cos (\mu ) \sin (\nu )
&\rho_{10}=e^{h-l} \sin (\mu ) \cos (\nu )-e^{l-h} \cos (\mu ) \sin (\nu )
\end{align}
$l$ and $h$ satisfy
\begin{align}
&\frac{\sinh (2 l)}{\sin (2 \nu )}=\frac{\sinh (2 h)}{\sin (2 \mu )}=\gamma
\end{align}
 and
\begin{align}
&g_1=\left(\sqrt{\gamma ^2 (-\cos (4 \mu ))+\gamma ^2+2}-\gamma  \sin (2 \mu )\right) \exp \left(\frac{1}{2} \left(\sinh ^{-1}(\gamma  \sin (2 \mu ))-\sinh ^{-1}(\gamma  \sin (2 \nu ))\right)\right),\\
&g_2=\frac{\sqrt{2} \exp \left(\frac{1}{2} \left(\sinh ^{-1}(\gamma  \sin (2 \nu ))-\sinh ^{-1}(\gamma  \sin (2 \mu ))\right)\right)}{\sqrt{2} \gamma  \sin (2 \mu )-\sqrt{\gamma ^2 (-\cos (4 \mu ))+\gamma ^2+2}}\\
&g_3=\exp \left(\frac{1}{2} \left(\sinh ^{-1}(\gamma  \sin (2 v))-\sinh ^{-1}(\gamma  \sin (2 u))\right)\right)=g_4^{-1}
\end{align}

\textcolor{red}{PLS do not read this sebsection, continue from 3.1.2}
\textcolor{green}{maybe add derivation as CPT map here and move this to appendix}

In this section we closely follow the derivation of \cite{manzano2018harnessing}. We are interested in studying the dynamics of a system in contact with an environment.

In what follows, we will use the subscripts $S$, $E$ and $T$ to identify the Hamiltonian, the Hilbert space and the density matrix of the system of interest (for which we would like to find the dynamics), the environment and the total (system + environment). We refer to $I$ to indicate the interaction Hamiltonian.
\textcolor{green}{add figure}

The Hilbert space and the Hamiltonian of the system + environment are
\begin{align}\label{hemiltoniansystenvtor}
&\mathcal{H}_T=\mathcal{H}_S\otimes \mathcal{H}_E,
&&H_T=H_S\otimes \id_E+\id_S\otimes H_E+ \alpha H_I,
\end{align}
where $H_S \in \mathcal{B}(\mathcal{H}_S)$, $H_E \in \mathcal{B}(\mathcal{H}_E)$ and $H_I \in \mathcal{B}(\mathcal{H}_T)$, $\mathcal{B}(\mathcal{H}_i)$ are the Hilbert spaces of the bounded operator. $\id_i$ are the identity operators. We will often omit the identity part, since it will be clear from the context. The parameter $\alpha$ is the strenght between the system and the environment.

We can write, without loss of generality, the interaction term as
\begin{align}
&H_I=\sum_k S_k \otimes E_k=\sum_k S_k^\dagger \otimes E_k^\dagger,
\end{align}
with $S_k$ and $E_k$ operators acting in the system and the environment. $H_I$ is Hermitian, but separately $S_k$ and $E_k$ are not.

Given the decomposition of the Hamiltonian \eqref{hemiltoniansystenvtor}, it is convenient to work in the interaction picture: both states and operators carry part of the time dependence and we put on top of the operators the symbol tilde ($\,\,\tilde{}\,\,\,$) to identify it.

The von-Neumann equation in this picture is
\begin{align}\label{vonneuman}
&\frac{d}{dt} \tilde{\rho}(t)=-i\, \alpha\, [\tilde{H}_I(t),\tilde{\rho}(t)]
\end{align}
and the integral form
\begin{align}\label{integralform}
\tilde{\rho}(t)= \tilde{\rho}(0)-i \alpha \int_0^t ds [\tilde H_I(s),\tilde{\rho}(s)].
\end{align}
We can insert  \eqref{integralform} into \eqref{vonneuman}  and get
\begin{align}
&\frac{d}{dt}\tilde\rho_T(t) = -i \alpha[\tilde H_i(t), \tilde\rho_T(t)]-\alpha^2 \int_0^t ds [\tilde H_I(t),[\tilde H_I(s),\tilde\rho_T(s)]].
\end{align}

Iterating this another time and neglecting term of order $\alpha^2$,
\begin{align}
&\frac{d}{dt}\tilde\rho_T(t) = -i \alpha[\tilde H_I(t), \tilde\rho_T(t)]-\alpha^2 \int_0^t ds [\tilde H_I(t),[\tilde H_I(s),\tilde\rho_T(t)]] .
\end{align}

This \textbf{approximation} (Markovian) assumes that the coupling constant $\alpha$ is small, the environment and the system are weakly coupled.

Since we are interested in the dynamical evolution of the restricted system, we can remove the contribution of the environmental degree of freedom by taking the partial trace\footnote{Note that this is independent from the picture we are working on.},
\begin{align}
\rho_S(t)=\Tr_E (\rho_T(t))=\sum_k \bra{e_k}\rho_T(t)\ket{e_k},
\end{align}
with $\ket{e_k}$ a basis of the environment Hilbert space.

We assume that $\Tr_E [\tilde H_I(t), \tilde\rho_T(t)]=0$.  and we obtain
\begin{align}\label{lindbladderivation}
&\frac{d}{dt}\tilde\rho_S(t) = -\alpha^2 \int_0^t ds \Tr_E[\tilde H_I(t),[\tilde H_I(s),\tilde\rho_T(t)]].
\end{align}

The fact $\Tr_E [\tilde H_I(t), \tilde\rho_T(t)]=0$ hides two extra \textbf{assumptions}. We have to impose that at initial time the system and the environment are uncorrelated $\tilde{\rho}_T(0)=\tilde{\rho}_S(0)\otimes \tilde{\rho}_E(0)$ and that the environment is in a thermal state with temperature $T$, $\tilde{\rho}_E(0)=\rho_{th}=e^{-H_E/T}/\Tr(e^{-H_E/T})$.

We notice that the right-hand site of \eqref{lindbladderivation} contains the density matrix of the total system. For arbitrary time we can write
\begin{align}
&\tilde{\rho}_T(t)=\tilde{\rho}(t)\otimes \tilde{\rho}_E(t)+\tilde{\rho}_{corr}(t),
\end{align}
$\tilde{\rho}_{corr}(t)$ is the entangled part of the total density matrix induced by the system-environment interaction. We \textbf{assume} that there is a strong separation in the timescale. The environment correlation $\tau_{corr}$ and relaxation $\tau_{rel}$ timescale are much faster than the timescale $\tau_0$ for the system to change due to the interaction with the environment. In particular, since $\tau_{corr}\ll \tau_0$, we can neglect $\tilde{\rho}_{corr}(t)$ at any time. Moreover, since $\tau_{rel}\ll \tau_0$, we can assume that the system is always interacting with a thermal environment $\tilde{\rho}_E(t)=\tilde{\rho}_{th}$. The environment, in fact, relaxes to thermodynamic equilibrium before any appreciable change in the system happens.

This approximation is very strong, however we are not assuming that there are no excitations in the reservoir caused by the reduced system. The time-scale of evolution are, in fact, very different and our description is valid on a  coarse-grained time scale. The assumption can also be formulated such that the environmental excitations are there, but they decay over characteristic time scale that are not resolved.

By using
\begin{align}
\tilde\rho_T(t)\approx\tilde\rho_s(t)\otimes \tilde\rho_{th},
\end{align}

we obtain
\begin{align}\label{lindbladd}
&\frac{d}{dt}\tilde\rho(t) = -\alpha^2 \int_0^t ds \Tr_E[\tilde H_I(t),[\tilde H_I(s),\tilde\rho_s(t)\otimes \tilde\rho_{th}]].
\end{align}

This is local in time, but since the time evolution of the reduced density matrix still depends on choice for the initial preparation time $t=0$, it is not yet a Markovian master equation. 

Due to the timescale separation, the memory kernel decays fast enough so the system forgets about its initial state and we are allowed to let the upper limit of the integral go to infinity. We also substitute $s\to t-s$.

In this way we obtain the Markovian quantum master equation called \textit{Redfield} equation

\begin{align}\label{lindbladeq22}
&\frac{d}{dt}\tilde\rho_S(t) = -\alpha^2 \int_0^\infty ds \Tr_E[\tilde H_I(t),[\tilde H_I(t-s),\tilde\rho_S(t)\otimes \tilde\rho_E]].
\end{align}
The dynamical behaviour over times of the order of magnitude of the correlation time $\tau_{corr}$ is however not resolved. The evolution is described in the sense on a coarse-grained time axis.

This equation does not warrant the positivity of the map, and it sometimes gives rise to density matrices that are non-positive. We need a further approximation to fix this.

The rotating wave \textbf{approximation}  involves an averaging over the rapidly oscillating terms. To do so, we use the spectrum of the superoperator $H\equiv [H, A], \forall A \in \mathcal{B}(\mathcal{H})$.

The eigenvectors of this superoperator form a complete basis of space $\mathcal{B}(\mathcal{H})$ and, therefore, we can expand the
system-environment operators in this basis
\begin{align}
S_i=\sum_\nu S_i(\nu),
\end{align}
where
\begin{align}
&[H_T,S_l(\nu)]=-\nu S_l (\nu),
&&[H_T,S_l^\dagger(\nu)]=\nu S_l^\dagger (\nu).
\end{align}

In the interaction picture, the system-environment interaction operator can be written as $\tilde{H_I}=e^{i t (H_s+H_E)} H_I e^{-i t (H_s+H_E)}$,
\begin{align}
&\tilde{H}_I=\sum_{l,\nu}e^{-i \nu t}S_l(\nu)\otimes \tilde{E_l}(t)=\sum_{l,\nu}e^{i \nu t}S_l^\dagger(\nu)\otimes \tilde{E_l}^\dagger(t).
\end{align}
We can expand the commutator of \eqref{lindbladeq22} and use the the spectral decomposition. We arrive at
\begin{align}
\dot{\tilde{\rho}}_S(t)=\sum_{\nu,\nu', k,l}\Big(e^{i(\nu'-\nu)t}\Gamma_{kl}(\nu)\Big[S_l(\nu)\tilde{\rho}_S(t),S_k^\dagger(\nu')\Big]+e^{i(\nu-\nu')t}\Gamma_{lk}^*(\nu)\Big[S_l(\nu')\tilde{\rho}_S(t),S_k^\dagger(\nu)\Big]\Big)
\end{align}
where
\begin{align}
\Gamma_{kl}(\nu)=\int_0^\infty ds\,e^{i\nu s}\Tr_E (\tilde{E}_k^\dagger (t)\tilde{E}_l(t-s)\tilde{\rho}_{th})= \int_0^\infty ds e^{i\nu s}\Tr_E (\tilde{E}_k^\dagger (s){E}_l\tilde{\rho}_{th}),
\end{align}
with $\tilde{E}_k(t)=e^{i H_E t}E_k e^{-i H_E t}$.

The terms with $|\nu'-\nu|\gg \alpha^2$ oscillate rapidly around zero before the system evolves appreciably due to the interaction with the environment. We only keep the term with $\nu=\nu'$ and we find

\begin{align}
\dot{\tilde{\rho}}_S(t)=\sum_{\nu\newline k,l}\Gamma_{kl}(\nu)\Big[S_l(\nu)\tilde{\rho}_S(t),S_k^\dagger(\nu)\Big]+\Gamma_{lk}^*(\nu)\Big[S_l(\nu),\tilde{\rho}_S(t)S_k^\dagger(\nu)\Big].
\end{align}
We can decompose the coefficients $\Gamma_{kl}$ into Hermitian and anti-Hermitian parts,
\begin{align}
&\Gamma_{kl}=\frac{1}{2}\gamma_{kl}(\nu)+ i \pi_{kl}(\nu),
\end{align}
\begin{align}
&\pi_{kl}=\frac{1}{2i}(\Gamma_{kl}(\nu)-\Gamma_{lk}^*(\nu)),
&&\gamma_{kl}(\nu)=\Gamma_{kl}(\nu)+\Gamma_{lk}^*(\nu)=\int_{-\infty}^\infty ds\,e^{i\nu s} \Tr_E \Big( \tilde{E}_k^\dagger (s)E_l \tilde{\rho}_{th}\Big)
\end{align}
and going back to the Schr\"odinger picture
\begin{align}
\dot{\rho}(t)=-i[H+\sum_{\nu k l}\pi_{kl}(\nu)S_k^\dagger(\nu)S_l(\nu),\rho(t)]+\sum_{\nu,\newline k,l} \gamma_{kl} (\nu) \Big( S_l(\nu) \rho(t) S_k^\dagger(\nu)-\frac{1}{2}\{\rho(t),S_k^\dagger(\nu)S_l(\nu)\}\Big),
\end{align}
where from now on we omit the index $S$ to identify the quantity corresponding to the system.

The coefficients $\gamma_{kl}(\nu)$ are positive semidefinite in all cases and they can be diagonalized by a unitary transformation leading to the Lindblad equation in the standard form

\begin{align}
\dot{\rho}(t)=-i[H,\rho(t)]+\sum_{i,\nu}  \Big( \ell_i(\nu) \rho(t) \ell_i^\dagger(\nu)-\frac{1}{2}\{\rho(t),\ell_i^\dagger(\nu)\ell_i(\nu)\}\Big),
\end{align}
where we neglected the second term in the commutator.

The $\ell$s operator are called jump operators and are related to the $S$. We first diagonalize $\gamma$ via a unitary transformation $\tau$, such that $d_i(\nu)=\sum_{kl}\tau_{ik}\gamma_{kl}(\nu)\tau_{il}^*$. The $\ell$ are then related to the $d_i$ via $\ell_i(\nu)=\sqrt{d_i(\nu)}\sum_l\tau_{il}S_l(\nu)$.

This dynamical evolution preserves the physical requirement of the density matrix: trace preserving and complete positive.

In the appendix \ref{DerivationLindblad}, we give the derivation of the Lindblad equation as a CPT generator.
\textcolor{green}{Maybe move that here and this in the appendix?}
